# Supplementary material for: Autonomous Improvement of Instruction Following Skills via Foundation Models
Source: arXiv:2407.20635 source file (2024-10-15)
Supplement: Supplementary file 1 [file appendix.tex]

action merging... (cite BC-Z)
